# Supplementary material for: Learning Discriminative Signed Distance Functions from Multi-scale Level-of-detail Features for 3D Anomaly Detection
Source: arXiv:2605.03437 source file (2026-05-06)
Supplement: Supplementary file 1 [file Supplementary_Material.tex]

% \textbf{Learning Discriminative Signed Distance Functions with Decoupled Level-of-detail Features for 3D Anomaly Detection—Supplementary Material}
%\input{Supplementary Material/results_Anomoly_O_AUPR}
\newpage
\begin{table*}[h]
  \centering
% \caption{O-AUROC performance of different methods on Real3D-AD across 40 categories, where best and second-place results are highlighted in red and blue, respectively.}
  \resizebox{0.95\textwidth}{!}{
    \begin{tabular}{c|cccccccccccccc}
    \toprule
    %\multicolumn{15}{c}{\textbf{O-AUROC}} \\
    %\midrule
    \textbf{Method} & \textbf{ashtray0} & \textbf{bag0} & \textbf{bottle0} & \textbf{bottle1} & \textbf{bottle3} & \textbf{bowl0} & \textbf{bowl1} & \textbf{bowl2} & \textbf{bowl3} & \textbf{bowl4} & \textbf{bowl5} & \textbf{bucket0} & \textbf{bucket1} & \textbf{cap0} \\
    \midrule
\textbf{BTF(Raw) (CVPR23’)} & 0.578 & 0.458 & 0.466 & 0.573 & 0.543 & 0.588 & 0.464 & 0.576 & 0.654 & 0.601 & 0.615 & 0.652 & 0.620 & 0.659 \\
\textbf{BTF(FPFH) (CVPR23’)} & 0.651 & 0.551 & 0.644 & 0.625 & 0.602 & 0.576 & 0.648 & 0.515 & 0.499 & 0.632 & 0.699 & 0.483 & 0.648 & 0.618 \\
\textbf{M3DM (CVPR23’)} & 0.632 & 0.642 & 0.763 & 0.674 & 0.451 & 0.525 & 0.515 & 0.630 & 0.635 & 0.571 & 0.601 & 0.609 & 0.507 & 0.564 \\
\textbf{PatchCore(FPFH) (CVPR22’)} & 0.445 & 0.608 & 0.615 & 0.677 & 0.579 & 0.548 & 0.545 & 0.611 & 0.620 & 0.575 & 0.541 & 0.604 & 0.565 & 0.585  \\
\textbf{PatchCore(PointMAE)  (CVPR22')} & \textcolor{blue}{0.679} & 0.601 & 0.545 & 0.645 & 0.651 & 0.562 & 0.611 & 0.456 & 0.556 & 0.601 & 0.585 & 0.541 & 0.642 & 0.561 \\
\textbf{CPMF (PR24’)} & 0.453 & 0.655 & 0.588 & 0.592 & 0.505 & 0.775 & 0.621 & 0.601 & 0.418 & 0.683 & 0.685 & 0.662 & 0.501 & 0.601  \\
\textbf{Reg3D-AD (NeurIPS23’)} & 0.588 & 0.608 & 0.632 & 0.695 & 0.474 & 0.494 & 0.515 & 0.495 & 0.441 & 0.624 & 0.555 & 0.632 & 0.714 & 0.693  \\
\textbf{IMRNet (CVPR24’)} & 0.612 & 0.665 & 0.558 & 0.702 & 0.648 & 0.481 & 0.504 & 0.681 & 0.614 & 0.630 & 0.652 & 0.578 & 0.732 & 0.711  \\
\textbf{PO3AD (CVPR25')} & \textcolor{red}{0.999} & \textcolor{blue}{0.809} & \textcolor{blue}{0.927} & \textcolor{blue}{0.959} & \textcolor{blue}{0.962} & \textcolor{blue}{0.946} & \textcolor{blue}{0.905} & \textcolor{blue}{0.888} & \textcolor{blue}{0.927} & \textcolor{red}{0.985} & \textcolor{blue}{0.904} & \textcolor{blue}{0.923} & \textcolor{blue}{0.882} & \textcolor{blue}{0.841}\\
\textbf{Ours} & \textcolor{red}{0.999} & \textcolor{red}{0.999} & \textcolor{red}{0.999} & \textcolor{red}{1.000} & \textcolor{red}{1.000} & \textcolor{red}{1.000} & \textcolor{red}{0.982} & \textcolor{red}{1.000} & \textcolor{red}{1.000} & \textcolor{blue}{0.976} & \textcolor{red}{0.991} & \textcolor{red}{0.981} & \textcolor{red}{0.922} & \textcolor{red}{0.934}\\

% \textbf{Reg2Inv(NIPS25')} & \textcolor{blue}{0.900} & \textcolor{red}{1.000} & \textcolor{red}{1.000} & \textcolor{red}{1.000} & \textcolor{red}{1.000} & \textcolor{red}{1.000} & 0.807 & 0.656 & 0.585 & 0.852 & 0.818 & 0.813 & \textcolor{red}{0.902} & 0.659
% \\

    \midrule
    \multicolumn{1}{c}{} &       &       &       &       &       &       &       &       &       &       &       &       &       &  \\
    \midrule
    \textbf{Method} & \textbf{cap3} & \textbf{cap4} & \textbf{cap5} & \textbf{cup0} & \textbf{cup1} & \textbf{eraser0} & \textbf{headset0} & \textbf{headset1} & \textbf{helmet0} & \textbf{helmet1} & \textbf{helmet2} & \textbf{helmet3} & \textbf{jar0} & \textbf{micro.} \\
    \midrule
\textbf{BTF(Raw) (CVPR23’)} & 0.612 & 0.515 & 0.653 & 0.601 & 0.701 & 0.425 & 0.379 & 0.515 & 0.559 & 0.388 & 0.615 & 0.526 & 0.428 & 0.613  \\
\textbf{BTF(FPFH) (CVPR23’)} & 0.579 & 0.545 & 0.593 & 0.585 & 0.651 & 0.719 & 0.531 & 0.523 & 0.568 & 0.721 & 0.588 & 0.564 & 0.479 & 0.662 \\
\textbf{M3DM (CVPR23’)} & 0.652 & 0.477 & 0.642 & 0.570 & \textcolor{blue}{0.752} & 0.625 & 0.632 & 0.623 & 0.528 & 0.627 & 0.636 & 0.458 & 0.555 & 0.464  \\
\textbf{PatchCore(FPFH) (CVPR22’)} & 0.457 & 0.655 & 0.725 & 0.604 & 0.586 & 0.584 & 0.701 & 0.601 & 0.525 & 0.630 & 0.475 & 0.494 & 0.499 & 0.332 \\
\textbf{PatchCore(PointMAE)  (CVPR22')} & 0.583 & \textcolor{blue}{0.721} & 0.542 & 0.642 & 0.710 & 0.801 & 0.515 & 0.423 & 0.633 & 0.571 & 0.496 & 0.611 & 0.463 & 0.652  \\
\textbf{CPMF (PR24’)} & 0.541 & 0.645 & 0.697 & 0.647 & 0.609 & 0.544 & 0.602 & 0.619 & 0.333 & 0.501 & 0.477 & 0.645 & 0.618 & 0.655  \\
\textbf{Reg3D-AD (NeurIPS23’)} & 0.711 & 0.623 & 0.770 & 0.531 & 0.638 & 0.424 & 0.538 & 0.617 & 0.600 & 0.381 & 0.618 & 0.468 & 0.601 & 0.614 \\
\textbf{IMRNet (CVPR24’)} & 0.702 & 0.658 & 0.502 & 0.455 & 0.627 & 0.599 & 0.701 & 0.656 & 0.697 & 0.615 & 0.602 & 0.575 & 0.760 & 0.552  \\
\textbf{PO3AD (CVPR25')} & \textcolor{red}{0.906} & \textcolor{red}{0.876} & \textcolor{blue}{0.801} & \textcolor{blue}{0.879} & \textcolor{red}{0.870} & \textcolor{blue}{0.995} & \textcolor{blue}{0.765} & \textcolor{blue}{0.914} & \textcolor{blue}{0.864} & \textcolor{blue}{0.961} & \textcolor{red}{0.934} & \textcolor{blue}{0.849} & \textcolor{blue}{0.915} & \textcolor{blue}{0.803}\\
\textbf{Ours} & \textcolor{blue}{0.730} & 0.688 & \textcolor{red}{0.853} & \textcolor{red}{0.999} & 0.523 & \textcolor{red}{0.999} & \textcolor{red}{1.000} & \textcolor{red}{0.999} & \textcolor{red}{0.926} & \textcolor{red}{0.991} & \textcolor{blue}{0.744} & \textcolor{red}{0.970} & \textcolor{red}{0.999} & \textcolor{red}{0.999} \\

% \textbf{Reg2Inv(NIPS25')} & \textcolor{red}{0.863} & 0.681 & \textcolor{blue}{0.902} & 0.733 & \textcolor{red}{0.933} & \textcolor{red}{1.000} & \textcolor{red}{1.000} & 0.843 & \textcolor{blue}{0.817} & \textcolor{blue}{0.986} & \textcolor{red}{0.875} & \textcolor{blue}{0.876} & \textcolor{red}{1.000} & \textcolor{red}{1.000}
% \\
    \midrule
    \multicolumn{1}{c}{} &       &       &       &       &       &       &       &       &       &       &       &       &       &  \\
    \midrule
    \textbf{Method} & \textbf{shelf0} & \textbf{tap0} & \textbf{tap1} & \textbf{vase0} & \textbf{vase1} & \textbf{vase2} & \textbf{vase3} & \textbf{vase4} & \textbf{vase5} & \textbf{vase7} & \textbf{vase8} & \textbf{vase9} & \textbf{Average} \\
    \midrule
\textbf{BTF(Raw) (CVPR23’)} & 0.624 & 0.535 & 0.594 & 0.562 & 0.441 & 0.413 & 0.717 & 0.428 & 0.615 & 0.547 & 0.416 & 0.482 & 0.549    \\
\textbf{BTF(FPFH) (CVPR23’)} & 0.611 & 0.610 & 0.575 & 0.641 & 0.655 & 0.569 & 0.652 & 0.587 & 0.472 & 0.592 & 0.624 & 0.638 & 0.598  \\
\textbf{M3DM (CVPR23’)} & 0.665 & 0.722 & 0.638 & \textcolor{blue}{0.788} & 0.652 & 0.615 & 0.551 & 0.526 & 0.633 & 0.648 & 0.463 & 0.651 & 0.603 \\
\textbf{PatchCore(FPFH) (CVPR22’)} & 0.504 & 0.712 & 0.684 & 0.645 & 0.623 & 0.801 & 0.481 & 0.777 & 0.515 & 0.621 & 0.515 & 0.660 & 0.588   \\
\textbf{PatchCore(PointMAE)  (CVPR22')} & 0.543 & 0.712 & 0.542 & 0.548 & 0.572 & 0.711 & 0.455 & 0.586 & 0.585 & 0.652 & 0.655 & 0.634 & 0.595    \\
\textbf{CPMF (PR24’)} & \textcolor{blue}{0.681} & 0.639 & 0.697 & 0.632 & 0.645 & 0.632 & 0.588 & 0.655 & 0.518 & 0.432 & 0.673 & 0.618 & 0.597  \\
\textbf{Reg3D-AD (NeurIPS23’)} & 0.675 & 0.676 & 0.599 & 0.615 & 0.468 & 0.641 & 0.651 & 0.505 & 0.588 & 0.455 & 0.629 & 0.574 & 0.584   \\
\textbf{IMRNet (CVPR24’)} & 0.625 & 0.401 & \textcolor{blue}{0.796} & 0.573 & 0.725 & 0.655 & 0.708 & 0.528 & 0.654 & 0.601 & 0.639 & 0.462 & 0.621 \\
\textbf{PO3AD (CVPR25')} & 0.680 & \textcolor{blue}{0.856} & 0.709 & 0.753 & \textcolor{blue}{0.789} & \textcolor{blue}{0.963} & \textcolor{blue}{0.902} & \textcolor{blue}{0.824} & \textcolor{blue}{0.879} & \textcolor{blue}{0.971} & \textcolor{blue}{0.833} & \textcolor{blue}{0.904} & \textcolor{blue}{0.881}\\
\textbf{Ours} & \textcolor{red}{0.811} & \textcolor{red}{0.921} & \textcolor{red}{0.951} & \textcolor{red}{0.847} & \textcolor{red}{0.976} & \textcolor{red}{0.999} & \textcolor{red}{0.926} & \textcolor{red}{0.916} & \textcolor{red}{0.999} & \textcolor{red}{0.999} & \textcolor{red}{0.956} & \textcolor{red}{0.934} & \textcolor{red}{0.936}\\
% \textbf{Reg2Inv(NIPS25')} & 0.577 & \textcolor{red}{0.948} & 0.804 & \textcolor{blue}{0.996} & 0.605 & \textcolor{red}{1.000} & \textcolor{blue}{0.845} & 0.818 & \textcolor{red}{1.000} & 0.643 & \textcolor{blue}{0.818} & \textcolor{red}{0.873} & 0.861
% \\
    \bottomrule
    \end{tabular}%
}
    \caption{The O-AUPR ($\uparrow$) performance of different methods on Anomaly-ShapeNet, where the best and second-place results are highlighted in \textcolor{red}{red} and \textcolor{blue}{blue}, respectively.}
  \label{results1}
\end{table*}

\section{More Experiment Results}
To further examine the performance of the proposed method, the object-level AUPR (Area Under the Precision-Recall curve) and pixel-level AUPR (Area Under the Precision-Recall curve) were introduced for evaluation.

\subsection{Results on Anomaly-ShapeNet}
Tables ~\ref{results1} and ~\ref{results2} report the anomaly detection and localization results of different methods on the Anomaly-ShapeNet dataset, respectively. The average O-AUPR of the proposed method reached 0.936, surpassing the second-best method by 5.5\%. To our knowledge, there are no publicly available P-AUPR results for the Anomaly-ShapeNet dataset. Nevertheless, our method achieved an average P-AUPR of 0.537, highlighting its effectiveness in anomaly detection across different data categories.
capability across different categories of data.
\begin{table*}[!ht]
  \centering
    % \caption{P-AUROC performance of different methods on Anomaly-ShapeNet across 40 categories, where best and second-place results are highlighted in red and blue, respectively.}
  \resizebox{0.95\textwidth}{!}{
    \begin{tabular}{c|cccccccccccccc}

    \midrule
    \textbf{Method} & \textbf{ashtray0} & \textbf{bag0} & \textbf{bottle0} & \textbf{bottle1} & \textbf{bottle3} & \textbf{bowl0} & \textbf{bowl1} & \textbf{bowl2} & \textbf{bowl3} & \textbf{bowl4} & \textbf{bowl5} & \textbf{bucket0} & \textbf{bucket1} & \textbf{cap0} \\
    \midrule
\textbf{Ours} & 0.365&0.678&0.896&0.157&0.050&0.942&0.590&0.211&0.804&0.591&0.670&0.052&0.793&0.885\\

% \textbf{Reg2Inv(NIPS25')} & 0.785 & {0.991} & {0.995} & 0.849 & 0.817 & {0.983} & 0.828 & 0.822 & 0.761 & 0.788 & 0.824 & 0.610 & 0.855 & 0.861\\

    \midrule
    \multicolumn{1}{c}{} &       &       &       &       &       &       &       &       &       &       &       &       &       &  \\
    \midrule
    \textbf{Method} & \textbf{cap3} & \textbf{cap4} & \textbf{cap5} & \textbf{cup0} & \textbf{cup1} & \textbf{eraser0} & \textbf{headset0} & \textbf{headset1} & \textbf{helmet0} & \textbf{helmet1} & \textbf{helmet2} & \textbf{helmet3} & \textbf{jar0} & \textbf{micro.} \\
    \midrule

\textbf{Ours} & 0.044&0.109&0.243&0.827&0.051&0.260&0.546&0.870&0.788&0.603&0.058&0.864&0.901&0.783\\

% \textbf{Reg2Inv(NIPS25')} & {0.945} & 0.864 & {0.970} & 0.798 & 0.881 & {0.980} & {0.946} & {0.970} & {0.925} & 0.906 & {0.891} & 0.956 & {0.982} & {0.992}\\
    \midrule
    \multicolumn{1}{c}{} &       &       &       &       &       &       &       &       &       &       &       &       &       &  \\
    \midrule
    \textbf{Method} & \textbf{shelf0} & \textbf{tap0} & \textbf{tap1} & \textbf{vase0} & \textbf{vase1} & \textbf{vase2} & \textbf{vase3} & \textbf{vase4} & \textbf{vase5} & \textbf{vase7} & \textbf{vase8} & \textbf{vase9} & \textbf{Average}\\
    \midrule
\textbf{Ours} & 0.119&0.819&0.651&0.347&0.592&0.867&0.737&0.169&0.715&0.825&0.785&0.252 &0.537 \\

% \textbf{Reg2Inv(NIPS25')} & 0.632 & {0.918} & 0.869 & {0.980} & 0.705 & {0.997} & 0.844 & {0.927} & 0.879 & 0.863 & {0.934} & {0.971} & 0.882\\
    \bottomrule
    \end{tabular}%
}
      \caption{The P-AUPR ($\uparrow$) performance of ours methods on Anomaly-ShapeNet}
  \label{results2}
\end{table*}
\begin{table*}[!ht]
  \centering
    % \caption{O-AUROC performance of different methods on Real3D-AD across 12 categories, where best and second-place results are highlighted in red and blue, respectively.}
  \resizebox{0.95\textwidth}{!}{
    \begin{tabular}{c|cccccccccccccc}
    \toprule
    %\multicolumn{14}{c}{\textbf{O-AUROC}}                                                                         &  \\
    %\midrule
    \textbf{Method} & \textbf{Airplane} & \textbf{Car} & \textbf{Candy} & \textbf{Chicken} & \textbf{Diamond} & \textbf{Duck} & \textbf{Fish} & \textbf{Gemstone} & \textbf{Seahorse} & \textbf{Shell} & \textbf{Starfish} & \textbf{Toffees} & \textbf{Average}  \\
    \midrule
\textbf{BTF(Raw) (CVPR23')} & 0.506 & 0.523 & 0.490 & 0.464 & 0.535 & \textcolor{red}{0.760} & 0.633 & 0.598 & 0.793 & \textcolor{blue}{0.751} & \textcolor{blue}{0.579} & 0.700 & 0.611    \\
\textbf{BTF(FPFH) (CVPR23')} & 0.659 & 0.653 & 0.638 & 0.814 & 0.677 & 0.620 & 0.638 & 0.603 & 0.567 & 0.434 & 0.557 & 0.505 & 0.614    \\
\textbf{M3DM((PointBERT) (CVPR23')} & 0.497 & 0.517 & 0.480 & 0.716 & 0.661 & 0.569 & 0.628 & \textcolor{blue}{0.628} & 0.491 & 0.638 & 0.573 & 0.569 & 0.581   \\
\textbf{M3DM(PointMAE) (CVPR23')} & 0.479 & 0.508 & 0.498 & 0.739 & 0.620 & 0.533 & 0.525 & \textcolor{red}{0.663} & 0.518 & 0.616 & 0.573 & 0.593 & 0.572  \\
\textbf{PatchCore(FPFH) (CVPR22')} & \textcolor{red}{0.852} & 0.611 & 0.553 & 0.872 & 0.569 & 0.506 & 0.642 & 0.411 & 0.508 & 0.573 & 0.491 & 0.506 & 0.591    \\
\textbf{PatchCore(FPFH+Raw)  (CVPR22')} & \textcolor{blue}{0.807} & \textcolor{blue}{0.766} & 0.611 & \textcolor{red}{0.885} & 0.767 & 0.560 & 0.844 & 0.411 & 0.763 & 0.553 & 0.473 & 0.559 & 0.667    \\
\textbf{PatchCore(PointMAE)  (CVPR22')} & 0.747 & 0.555 & 0.576 & 0.864 & 0.801 & 0.488 & 0.720 & 0.444 & 0.546 & 0.590 & 0.561 & 0.708 & 0.633   \\
\textbf{Reg3D-AD (NeurIPS23’)} & 0.703 & 0.753 & \textcolor{blue}{0.824} & \textcolor{blue}{0.884} & 0.884 & 0.588 & 0.939 & 0.454 & 0.787 & 0.646 & 0.491 & 0.721 & 0.723    \\
\textbf{Group3AD (MM24')} & 0.757 & 0.706 & \textcolor{red}{0.837} & 0.674 & \textcolor{blue}{0.932} & 0.612 & \textcolor{blue}{0.981} & 0.533 & \textcolor{blue}{0.842} & 0.648 & 0.567 & \textcolor{blue}{0.785} & \textcolor{blue}{0.740}    \\

\textbf{Ours} & 0.599 & \textcolor{red}{0.974} & 0.816 & 0.849 & \textcolor{red}{0.965} & \textcolor{blue}{0.717} & \textcolor{red}{0.982} & 0.617 & \textcolor{red}{0.967} & \textcolor{red}{0.848} & \textcolor{red}{0.620} & \textcolor{red}{0.943} & \textcolor{red}{0.824}
\\

% \textbf{Reg2Inv(NIPS25')} & 0.818 & 0.758 & \textcolor{red}{1.000} & \textcolor{red}{0.944} & \textcolor{red}{1.000} & 0.750 & 0.672 & \textcolor{red}{0.735} & 0.532 & 0.692 & \textcolor{red}{0.841} & 0.626 & 0.780\\

    \bottomrule
    \end{tabular}%
}
    \caption{The O-AUPR ($\uparrow$) performance of different methods on Real3D-AD, where the best and second-place results are highlighted in \textcolor{red}{red} and \textcolor{blue}{blue}, respectively}
  \label{results3}
\end{table*}

\begin{table*}[!ht]
  \centering
    % \caption{P-AUROC performance of different methods on Real3D-AD across 12 categories, where best and second-place results are highlighted in red and blue, respectively.}
  \resizebox{0.95\textwidth}{!}{
    \begin{tabular}{c|cccccccccccccc} 
    \midrule
    \textbf{Method} & \textbf{Airplane} & \textbf{Car} & \textbf{Candy} & \textbf{Chicken} & \textbf{Diamond} & \textbf{Duck} & \textbf{Fish} & \textbf{Gemstone} & \textbf{Seahorse} & \textbf{Shell} & \textbf{Starfish} & \textbf{Toffees} & \textbf{Average} \\
    \midrule
\textbf{BTF(Raw) (CVPR23')} & 0.012 & 0.014 & 0.025 & 0.049 & 0.032 & 0.020 & 0.017 & 0.014 & 0.031 & 0.011 & 0.017 & 0.016 & 0.022    \\
\textbf{BTF(FPFH) (CVPR23')} & \textcolor{blue}{0.027} & 0.028 & 0.118 & 0.044 & 0.239 & \textcolor{red}{0.068} & 0.036 & \textcolor{blue}{0.075} & 0.027 & 0.018 & 0.034 & 0.055 & 0.064  \\
\textbf{M3DM((PointBERT) (CVPR23')} & 0.007 & 0.017 & 0.016 & \textcolor{blue}{0.377} & 0.038 & 0.011 & 0.039 & 0.017 & 0.028 & 0.021 & 0.040 & 0.018 & 0.052    \\
\textbf{M3DM(PointMAE) (CVPR23')} & 0.007 & 0.018 & 0.016 & 0.310 & 0.033 & 0.011 & 0.025 & 0.018 & 0.030 & 0.022 & 0.040 & 0.021 & 0.046   \\
\textbf{PatchCore(FPFH) (CVPR22')} & \textcolor{blue}{0.027} & 0.034 & \textcolor{blue}{0.142} & 0.040 & 0.273 & \textcolor{blue}{0.055} & 0.052 & \textcolor{red}{0.093} & 0.031 & 0.031 & 0.037 & 0.040 & 0.071  \\
\textbf{PatchCore(FPFH+Raw)  (CVPR22')} & 0.016 & 0.160 & 0.092 & 0.045 & \textcolor{blue}{0.363} & 0.034 & 0.266 & 0.066 & \textcolor{blue}{0.291} & 0.049 & 0.035 & 0.055 & 0.123    \\
\textbf{PatchCore(PointMAE)  (CVPR22')} & 0.016 & 0.069 & 0.020 & 0.052 & 0.107 & 0.008 & 0.201 & 0.008 & 0.071 & 0.043 & 0.046 & 0.055 & 0.058    \\
\textbf{Reg3D-AD (NeurIPS23’)} & 0.017 & 0.135 & 0.109 & 0.044 & 0.191 & 0.010 & 0.437 & 0.016 & 0.182 & 0.065 & 0.039 & 0.067 & 0.109    \\
\textbf{Group3AD (MM24')} & 0.018 & \textcolor{red}{0.174} & 0.122 & 0.068 & 0.287 & 0.016 & \textcolor{blue}{0.448} & 0.009 & 0.24 & \textcolor{blue}{0.067} & \textcolor{blue}{0.056} & \textcolor{blue}{0.134} & \textcolor{blue}{0.137}  \\

\textbf{Ours} & \textcolor{red}{0.050} & \textcolor{blue}{0.167} & \textcolor{red}{0.485} & \textcolor{red}{0.508} & \textcolor{red}{0.436} & 0.048 & \textcolor{red}{0.577} & 0.039 & \textcolor{red}{0.715} & \textcolor{red}{0.321} & \textcolor{red}{0.127} & \textcolor{red}{0.445} & \textcolor{red}{0.326}
\\

% \textbf{Reg2Inv(NIPS25')} & {0.923} & {0.944} & {0.969} & {0.910} & {0.979} & {0.937} & 0.846 & {0.907} & 0.645 & {0.906} & {0.840} & 0.737 & {0.878}\\

    \bottomrule
    \end{tabular}%
}
    \caption{The P-AUPR ($\uparrow$) performance of different methods on Real3D-AD,where the best and second-place results are highlighted in \textcolor{red}{red} and \textcolor{blue}{blue}, respectively}
  \label{results11}
\end{table*}

\subsection{Experimental Results on Real3D-AD}
Tables~\ref{results3} and ~\ref{results11} show the performance of different methods on the Real3D-AD dataset. The proposed method yielded an average O-AUPR of 0.824 and an average P-AUPR of 0.326, outperforming the best comparison method by 8.4\% and 18.9\%, respectively. These results further verify the superiority of the proposed method for high-precision point clouds.

\section{More Ablation Studies}
\subsection{Effectiveness of the NPG Module} 
To further verify the effectiveness of the proposed Noisy Points Generation (NPG) module, we replaced it with the method of random noise and Norm-AS proposed in PO3AD ~\cite{PO3AD}. The experimental results on the Real3D-AD dataset are shown in Table $\ref{AnomalyGeneration}$.

 \begin{table}[htbp]
  \centering
  \resizebox{0.95\columnwidth}{!}{
    \begin{tabular}{c|ccc}
    \toprule
    \textbf{Method} & Random noise & Norm-AS & NPG (Ours)\\
    \midrule
    O-AUROC &0.659&0.735 &0.859\\
    P-AUROC & 0.557&0.539 &0.852\\
    \bottomrule
    \end{tabular}%
}
   \caption{Experimental results with different anomaly generation methods. }
  \label{AnomalyGeneration}
\end{table}

The method of random noise generates points that are randomly distributed in point cloud space. As shown in $\ref{AnomalyGeneration}$, the performance of the proposed method with random noise is significantly lower than that with the NPG module. This is because unstructured and irregular random points lack geometric correlation with the point cloud surface and cannot simulate the distributions of realistic anomalies.

Norm-AS is an anomaly synthesis method proposed by PO3AD~\cite{PO3AD}, whose core design concept is to generate local pseudo-anomalies through normal vectors. Although this method can realize the anomaly synthesis function, its performance is still inferior to that of the NPG module. The fundamental reason lies in the fact that our proposed method relies on the global surface modeling technology of point clouds, which requires the construction of a complete noise distribution that not only covers the local near-surface area but also includes the global space. However, the local pseudo-anomalies generated by Norm-AS are difficult to meet this requirement.

\subsection{Effectiveness of the MLF Module}
To verify the superiority of the proposed Multi-scale Level-of-detail Feature (MLF) module in capturing multi-scale geometric features, we conducted comparative experiments on the Real3D-AD dataset by replacing the MLF module with three alternative feature extraction methods, namely FPFH~\cite{BTF}, MLP~\cite{PO3AD}, and PointMAE~\cite {pointmae}. The results are shown in Table~\ref{Feature1}.

As shown in Table~\ref{Feature1}, the proposed method with the MLF module achieved the highest O-AUROC and P-AUROC among all compared methods.
FPFH relies on local geometric descriptors and lacks the ability to extract global structural information. MLP only performs feature mapping and fails to explore correlations between features at different scales. Although PointMAE can extract robust and generalized features through pre-training and masking strategies, it struggles to balance the capture of global context and local fine-grained features. In contrast, the MLF module can accurately capture both global shape structure and local details simultaneously by extracting multi-scale features, thus achieving superior performance in 3D anomaly detection.
 \begin{table}[htbp]
  \centering
  \resizebox{0.95\columnwidth}{!}{
    \begin{tabular}{c|cccc}
    \toprule
    \textbf{Feature} & FPFH& MLP & PointMAE & MLF (Ours)\\
    \midrule
    O-AUROC &0.559&0.778 &0.668&0.859\\
    P-AUROC & 0.457&0.745 &0.589&0.852\\
    \bottomrule
    \end{tabular}%
    }
   \caption{Performance of the proposed method with different feature extractors.}
  \label{Feature1}
\end{table}

\section{More Parameter Sensitivity Analysis}
\textbf{The influence of parameter $\alpha$.} 
To further examine the effect of the sampling ratio $\alpha=(\alpha_\text{surf}, \alpha_\text{near}, \alpha_\text{uni})$, the proposed method with extremely imbalanced ratios was investigated, and the results are summarized in Table~\ref {NoiseParameter}.

% As shown in Table~\ref {NoiseParameter}, the proposed method with only surface points degraded dramatically, with an 

As shown in Table~\ref {NoiseParameter}, when only surface points are used ($\alpha$ = 2:0:0), the model performance degrades significantly in both O-AUROC and P-AUROC, and the latter is even close to the performance of random guessing. Nevertheless, when increasing the ratio of near-surface points, the AUROC and P-AUROC performance improved by 2.0\% and 4.0\%, respectively. Meanwhile, increasing the ratio of uniform points also enhanced performance, but the improvement was less significant than that achieved by increasing the proportion of near-surface points. The reasons for these results may be that near-surface points provide discriminative feature information, while uniform points offer global spatial distribution information. Both types of information are beneficial for training anomaly detection models. However, excessively introducing uniform points may confuse model learning. Therefore, the sampling ratio is set to $\alpha=(2, 2, 1)$, which well balances the effects of different types of points.

 \begin{table}[htbp]
  \centering
  \resizebox{0.95\columnwidth}{!}{
    \begin{tabular}{c|cccccc}
    \toprule
    \textbf{$\alpha$} & 2:0:0 & 2:1:0 & 2:2:0 & 2:2:1 & 2:0:1 & 2:0:2 \\
    \midrule
    O-AUROC & 0.581&0.804&0.839& 0.859& 0.761& 0.795\\
    P-AUROC & 0.501&0.817&0.812& 0.852& 0.703& 0.757 \\
    \bottomrule
    \end{tabular}%
 }
   \caption{Effect on performance under extremely imbalanced sampling ratios. }
  \label{NoiseParameter}
\end{table}

\section{Result Visualization}
\subsection{Visualizations of Generated Points}
% Fig.~\ref{visNoisy3} visualizes the surface points $P_\text{surf}$, near-surface noisy points $P_\text{near}$, and uniform noisy points $P_\text{uni}$ generated by our Noisy Points Generation (NPG) module. 

%一种类型一种类型的解释，首先说表面点（说明他是用来替换原点云的），然后讲近表面，再说均匀点
Fig.~\ref{visNoisy3} visualizes the surface points $P_\text{surf}$, near-surface noisy points $P_\text{near}$, and uniform noisy points $P_\text{uni}$ generated by our Noisy Points Generation (NPG) module, respectively.
Specifically, the surface points $P_\text{surf}$ are sampled with the probability proportional to the area of the triangular mesh and are relatively uniformly distributed on the surface of the point clouds. The near-surface noisy points $P_\text{near}$ are obtained by adding Gaussian noise to the surface points, and the uniform noisy points are uniformly sampled within the 3D point cloud space.

It can be seen that the near-surface noisy points $P_\text{near}$ (yellow color) adhere closely to the surface of the input point cloud, and this characteristic effectively limits the distribution of normal points and also provides discriminative information for the training of anomaly detection models. Meanwhile, the uniform noisy points $P_\text{uni}$ (gray color) are uniformly sampled within the normalized 3D space $\mathbb{B}=[-1,1]^3$. This sampling method enables noisy points to fill the regions not covered by the near-surface points. The uniform characteristic further enhances the model's ability to detect anomalies in different scales.

\begin{figure*}[ht]
  \centering
  % \columnwidth textwidth
    \includegraphics[width=\linewidth]{Supplementary Material/visNoisy4.pdf}
  \caption{Visualization of the generated points on the Real3D dataset, with the blue, yellow, and gray points representing the surface points $P_\text{surf}$, near-surface noisy points $P_\text{near}$, and uniform noisy points $P_\text{uni}$, respectively.}
  \label{visNoisy3}
  
\end{figure*}
\begin{figure*}[ht]
  \centering
  % \columnwidth textwidth
  \includegraphics[width=\linewidth]{Supplementary Material/SDF_vis.pdf}
  %\caption{Visualization of 3D shape results of different sampling methods via the SDF model on the Real3D dataset.}
  \caption{Visualization of the distributions and the SDF values of the original and generated point clouds on the Real3D dataset, with higher red color indicating larger SDF values.}
  \label{visSDF}
\end{figure*}

\subsection{Visualizations of Point Distribution and the Learned SDF}
%首先描述现实，用生成的点替换原来的点。然后说为了体现生成点的优势，比较两者的点云和SDF的差异。
%首先分析原点云和生成点云的差异，说明生成点云的优势
% %再分析从两个不同点云上学到的SDF的差异，体现原点云会存在较大误差，并分析原因。
To mitigate the non-uniformity and sparsity of the original input point clouds, surface points are generated using the proposed NPG model. These points, rather than the original points, serve as the normal points for training the discriminative SDF network. To illustrate the advantages of the generated surface points over the original input points, their point distribution and corresponding SDF values are visualized in Figure \ref{visSDF}.

As shown in Figure \ref{visSDF}, the original point clouds (the first row) exhibit local unevenness, and their SDF values (the third row) also have relatively large errors (red points within the white bounding box). In contrast, the generated surface points (the second row) are distributed more uniformly on the surface of the point clouds, and their SDF values (the fourth row) tend toward 0. These results demonstrate the superiority of the generated surface points in learning the surface representation of point clouds using the discriminative SDF networks.

\section{Robustness to Noisy Data}
In practical application scenarios, the complexity of the environment and the instability of devices often lead to noise interference in scanned point clouds. To evaluate the robustness of the proposed method to noisy data, experiments were conducted on the Real3D dataset, where Gaussian noise with a standard deviation of 0, 0.001, 0.003, 0.005, or 0.01 was injected into test samples (a standard deviation of 0 indicates noise-free data). The experimental results are in Figure~\ref {Noise standard deviation}.

Notably, as the noise standard deviation increases, the model performance degrades moderately. Moreover, even in its worst-case noise scenario, the proposed method still outperforms other comparative methods that use clean data without injecting noise. These empirical findings highlight the robustness of our approach to noisy data.

\begin{figure}[ht]
  \centering
  % \columnwidth textwidth
  \includegraphics[width=\columnwidth]{AAAI2026_Xiaohaibo/Supplementary Material/Noise.pdf}
  \caption{Robustness of the proposed method to test noise.}
  %\caption{The impact of testing noise with different standard deviations on O-AUROC and P-AUROC.}
  \label{Noise standard deviation}
\end{figure}
