# Supplementary material for: Learning Discriminative Signed Distance Functions from Multi-scale Level-of-detail Features for 3D Anomaly Detection
Source: arXiv:2605.03437 source file (2026-05-06)
Supplement: Supplementary file 3 [file results_Anomoly_P_AUPR.tex]

\begin{table*}[!ht]
  \centering
    % \caption{P-AUROC performance of different methods on Anomaly-ShapeNet across 40 categories, where best and second-place results are highlighted in red and blue, respectively.}
  \resizebox{0.95\textwidth}{!}{
    \begin{tabular}{c|cccccccccccccc}

    \midrule
    \textbf{Method} & \textbf{ashtray0} & \textbf{bag0} & \textbf{bottle0} & \textbf{bottle1} & \textbf{bottle3} & \textbf{bowl0} & \textbf{bowl1} & \textbf{bowl2} & \textbf{bowl3} & \textbf{bowl4} & \textbf{bowl5} & \textbf{bucket0} & \textbf{bucket1} & \textbf{cap0} \\
    \midrule
\textbf{Ours} & 0.365&0.678&0.896&0.157&0.050&0.942&0.590&0.211&0.804&0.591&0.670&0.052&0.793&0.885\\

% \textbf{Reg2Inv(NIPS25')} & 0.785 & {0.991} & {0.995} & 0.849 & 0.817 & {0.983} & 0.828 & 0.822 & 0.761 & 0.788 & 0.824 & 0.610 & 0.855 & 0.861\\

    \midrule
    \multicolumn{1}{c}{} &       &       &       &       &       &       &       &       &       &       &       &       &       &  \\
    \midrule
    \textbf{Method} & \textbf{cap3} & \textbf{cap4} & \textbf{cap5} & \textbf{cup0} & \textbf{cup1} & \textbf{eraser0} & \textbf{headset0} & \textbf{headset1} & \textbf{helmet0} & \textbf{helmet1} & \textbf{helmet2} & \textbf{helmet3} & \textbf{jar0} & \textbf{micro.} \\
    \midrule

\textbf{Ours} & 0.044&0.109&0.243&0.827&0.051&0.260&0.546&0.870&0.788&0.603&0.058&0.864&0.901&0.783\\

% \textbf{Reg2Inv(NIPS25')} & {0.945} & 0.864 & {0.970} & 0.798 & 0.881 & {0.980} & {0.946} & {0.970} & {0.925} & 0.906 & {0.891} & 0.956 & {0.982} & {0.992}\\
    \midrule
    \multicolumn{1}{c}{} &       &       &       &       &       &       &       &       &       &       &       &       &       &  \\
    \midrule
    \textbf{Method} & \textbf{shelf0} & \textbf{tap0} & \textbf{tap1} & \textbf{vase0} & \textbf{vase1} & \textbf{vase2} & \textbf{vase3} & \textbf{vase4} & \textbf{vase5} & \textbf{vase7} & \textbf{vase8} & \textbf{vase9} & \textbf{Average}\\
    \midrule
\textbf{Ours} & 0.119&0.819&0.651&0.347&0.592&0.867&0.737&0.169&0.715&0.825&0.785&0.252 &0.537 \\

% \textbf{Reg2Inv(NIPS25')} & 0.632 & {0.918} & 0.869 & {0.980} & 0.705 & {0.997} & 0.844 & {0.927} & 0.879 & 0.863 & {0.934} & {0.971} & 0.882\\
    \bottomrule
    \end{tabular}%
}
      \caption{The P-AUPR ($\uparrow$) performance of ours methods on Anomaly-ShapeNet}
  \label{results2}
\end{table*}
